# Supplementary material for: A Comparative Study of Limiting Strategies in Discontinuous Galerkin Schemes for the $M_1$ Model of Radiation Transport
Source: arXiv:1706.10174 source file (2017-06-30)
Supplement: Supplementary file 1 [file additionalnumerics.tex]

%\section{Implementation Details}
%\label{sec:details}
%
\section{Numerical Results}
\label{sec:numerical_results}
In this section, we compare the performance of the RKDG schemes on unstructured triangular meshes
and uniform rectangular meshes for various combinations of limiters. Specifically we consider the limiter combinations given in Table~\ref{tab:LimiterCombinations}.
\begin{table}[h]
\centering
\begin{tabular}{l l}
Abbr. & Explanation\\
\midrule
SL$M$$\square/\triangle$ & Slope limiter in primitive variables with the constant $M$ specified\\
CL$M$$\square/\triangle$ & Slope limiter in characteristic variables with the constant $M$ specified\\
SRL$M$$\square/\triangle$ & Slope limiter in primitive variables + realizability limiter\\
CRL$M$$\square/\triangle$ & Slope limiter in characteristic variables + realizability limiter\\
\end{tabular}
\caption{Abbreviation of limiter combinations. Setting $M=\infty$ is equivalent to disabling the slope limiter. $\square$ and $\triangle$ correspond to the rectangular and triangular meshes, respectively.}
\label{tab:LimiterCombinations}
\end{table}

A complete characterization and discussion of the first 4 test cases is presented
in the paper. The last test case is an additional test case on the collision of two beams.

\subsection{Line Source}
\begin{itemize}
\item Domain: $[-0.5,0.5]^2$ with $h =0.004$
\item Time $T=0.45$
\item Parameters: $\sigma_a=\sigma_s=0$, $q^{(0)}=0$, $q^{(1)}=0$
\item Initial condition: $\psi^{(0)}(x,y) = \max(\exp(-10\frac{x^2+y^2}{\sigma^2}),10^{-4})$ with $\sigma=0.02$, $\psi^{(1)}(x,y)=0$
\item Boundary conditions are Dirichlet conditions equal to the initial conditions. Because the signal does not reach the boundary, these conditions do not influence the result.
\end{itemize}

\begin{figure}[h]

\centering
\externaltikz{LinesourceAdd3}{\input{Images/LinesourceAdd3}}
\caption{Line source: comparison of unlimited solution with and without realizability limiter.}
\label{fig:linesource3}
\end{figure}

\begin{figure}[h]

\centering
\externaltikz{LinesourceAdd}{\input{Images/LinesourceAdd1}}
\caption{Line source: comparison of primitive and characteristic slope limiter.}
\label{fig:linesource}
\end{figure}

\begin{figure}[h]

\centering
\externaltikz{LinesourceAdd2}{\input{Images/LinesourceAdd2}}
\caption{Line source: comparison of primitive and characteristic slope limiter with realizability limiter.}
\label{fig:linesource2}
\end{figure}

\clearpage
\subsection{Homogeneous Disk}
\begin{itemize}
\item Domain: $[-5,5]^2$ with $h=0.05$
\item Time: 3.75
\item Parameters: Let $D$ be the unit disk $D=\{ (x,y):\ x^2+y^2\leq 1\}$. Set $\sigma_s=0$; $\sigma_a=10$ on $D$, zero otherwise; source $q^{(0)}=1$ on $D$, zero otherwise; $q^{(1)} = 0$
\item Initial condition: $\psi^{(0)}=0$
\item Boundary conditions: vacuum
\end{itemize}

\begin{figure}[h]

\centering
\externaltikz{HomDiskAdd3}{\input{Images/HomDiskAdd3}}
\caption{Homogeneous disk: comparison of unlimited solution with and without realizability limiter.}
\label{fig:homdisk3}
\end{figure}

\begin{figure}[h]

\centering
\externaltikz{HomDiskAdd}{\input{Images/HomDiskAdd1}}
\caption{Homogeneous disk: comparison of primitive and characteristic slope limiter.}
\label{fig:homdisk}
\end{figure}

\begin{figure}[h]

\centering
\externaltikz{HomDiskAdd2}{\input{Images/HomDiskAdd2}}
\caption{Homogeneous disk: comparison of primitive and characteristic slope limiter with realizability limiter.}
\label{fig:homdisk2}
\end{figure}

\clearpage
\subsection{Flash}
\begin{itemize}
\item Domain: $[-10,10]^2$ with $h =0.06$
\item Time: 6
\item Parameters: Let $D$ be unit disk with radius five $D=\{ (x,y):\ x^2+y^2\leq 25\}$. Set $\sigma_s=0$; $\sigma_a=0$; source $q^{(0)}=0$, $q^{(1)} = 0$
\item Initial condition: $\psi^{(0)}=1$, $\psi^{(1)}_x=0.9$, $\psi^{(1)}_y=0$ on $D$, zero otherwise
\item Boundary conditions: vacuum
\end{itemize}

\begin{figure}[h]

\centering
\externaltikz{FlashAdd3}{\input{Images/FlashAdd3}}
\caption{Flash: comparison of unlimited solution with and without realizability limiter.}
\label{fig:flash3}
\end{figure}

\begin{figure}[h]

\centering
\externaltikz{FlashAdd}{\input{Images/FlashAdd1}}
\caption{Flash: comparison of primitive and characteristic slope limiter.}
\label{fig:flash}
\end{figure}
\begin{figure}[h]

\centering
\externaltikz{FlashAdd2}{\input{Images/FlashAdd2}}
\caption{Flash: comparison of primitive and characteristic slope limiter with realizability limiter.}
\label{fig:flash2}
\end{figure}

\clearpage
\subsection{Shadow}
\begin{itemize}
\item Domain: $[0,12]\times[0,6]$, $h=0.04$
\item Time: until steady state
\item Parameters: Let $O$ be the obstacle $O=[2,3]\times [0,2]$. Set $\sigma_s=0$; $\sigma_a=50$ on $O$, zero otherwise; source $q^{(0)}=0$; $q^{(1)} = 0$
\item Initial condition: $\psi^{(0)}=0$
\item Boundary conditions: top/bottom reflective, right vacuum, left Dirichlet with $\psi^{(0)}=1$, $\psi^{(1)}_x=0.99$, $\psi^{(1)}_y=0$
\end{itemize}

\begin{figure}[h]

\centering
\externaltikz{ShadowAdd3}{\input{Images/ShadowAdd3}}
\caption{Shadow: comparison of unlimited solution with and without realizability limiter.}
\label{fig:shadow3}
\end{figure}

\begin{figure}[h]

\centering
\externaltikz{ShadowAdd}{\input{Images/ShadowAdd1}}
\caption{Line source: comparison of primitive and characteristic slope limiter.}
\label{fig:shadow}
\end{figure}

\begin{figure}[h]

\centering
\externaltikz{ShadowAdd2}{\input{Images/ShadowAdd2}}
\caption{Line source: comparison of primitive and characteristic slope limiter with realizability limiter.}
\label{fig:shadow2}
\end{figure}

\clearpage

\subsection{Two Beams}
\begin{itemize}
\item Domain: $[0,7]\times[0,7]$, $h=0.05$
\item Time: 7
\item Parameters: $\sigma_a=\sigma_s=0$, $q^{(0)}=0$, $q^{(1)}=0$
\item Initial condition: $\psi^{(0)}=10^{-4}$, $\psi^{(1)}=0$
\item Boundary conditions: left $\psi^{(0)}=100$, $\psi^{(1)}_x=99.9$, $\psi^{(1)}_y=0$ in $0\times [3,4]$, bottom $\psi^{(0)}=100$, $\psi^{(1)}_x=0$, 
    $\psi^{(1)}_y=99.9$ in $[3,4]\times 0$,  else $\psi^{(0)}=10^{-4}$, $\psi^{(1)}=0$
\end{itemize}

\begin{figure}[h]

\centering
\externaltikz{TwoBeamsAdd3}{\input{Images/TwoBeamsAdd3}}
\caption{Two beams: comparison of unlimited solution with and without realizability limiter.}
\label{fig:Twobeams3}
\end{figure}
In Figure~\ref{fig:Twobeams3} we observe that in the absence of any limiting the numerical solution on the triangular unstructured mesh is unstable
and completely blows up. While the solution on the rectangular mesh does not completely blow up, it is highly oscillatory and loses realizability
on parts of the domain. Adding the realizability limiter stabilizes both numerical solutions; however, there are visible oscillations in 
the region where the beams collide.

\begin{figure}[h]

\centering
\externaltikz{TwoBeamsAdd}{\input{Images/TwoBeamsAdd1}}
\caption{Two beams: comparison of primitive and characteristic slope limiter.}
\label{fig:Twobeams}
\end{figure}
In Figure~\ref{fig:Twobeams} we note that limiting in the primitive or characteristic variables results in a solution that is not realizable on parts of the domain.
In the case of the unstructured triangular mesh the limiting in primitive variables results in an asymmetric solution. While
limiting in the characteristic variables leads to a better solution on both meshes, realizability cannot be guaranteed on the whole domain.
\begin{figure}[h]

\centering
\externaltikz{TwoBeamsAdd2}{\input{Images/TwoBeamsAdd2}}
\caption{Two beams: comparison of primitive and characteristic slope limiter with realizability limiter.}
\label{fig:Twobeams2}
\end{figure}

Finally in Figure~\ref{fig:Twobeams2}, the combination of limiting in characteristic variables plus
the realizability limiter leads to a superior solution on both meshes. However, we point out that in this test case
on the unstructured mesh, the numerical solution does not maintain a perfect symmetry when the beams collide. We have observed
that this is in part due to the fact that the transformations to and from the characteristic variables are ill conditioned
at the point when the beams collide.
